# Supplementary material for: Mean skewness measures
Source: arXiv:1912.06996 source file (2019-12-17)
Supplement: Supplementary file 1 [file Appendix.tex]

\appendix
%-------------------------------------------------%
\section{Appendix} \label{sec:Appendix}
%-------------------------------------------------%

%---------------------------------------------------------------------%
\subsection{$\cov(S_p,S_q)$} \label{sec:Cov_spsq}
%---------------------------------------------------------------------%
\begin{align*}
&\cov(s_p,s_q)\\
&= \cov(x_{1-p} + x_p -2 x_{0.5}, x_{1-q} + x_q - 2 x_{0.5})\\
&= E\{[(x_{1-p}- \hat{x}_{1-p}) + (x_p - \hat{x}_p) - 2(x_{0.5} - \hat{x}_{0.5})][(x_{1-q}- \hat{x}_{1-q}) + (x_q - \hat{x}_q) - 2(x_{0.5} - \hat{x}_{0.5})] \}\\
&= \cov(x_{1-p}, x_{1-q}) + \cov(x_{1-p}, x_q) + \cov(x_p, x_{1-q}) + \cov(x_p, x_q)- 2\cov(x_{1-p},x_{0.5}) \\
&  \;\;\;\;\;\;  - 2  \cov(x_p, x_{0.5}) - 2  \cov(x_{0.5},x_{1-q}) - 2  \cov(x_{0.5},x_q) + 4 \var(x_{0.5})
\end{align*}
%---------------------------------------------------------------------%
\subsection{$\cov(S_p,R_{1,q})$} \label{sec:Cov_sprq}
%---------------------------------------------------------------------%
\begin{align*}
&\cov(s_p,r_{1q})\\
&= \cov(x_{1-p} + x_p -2x_{0.5}, x_{1-q} - x_q)  \\ 
&= E\{[(x_{1-p}- \hat{x}_{1-p}) + (x_p - \hat{x}_p) - 2(x_{0.5} - \hat{x}_{0.5})]  [(x_{1-q}- \hat{x}_{1-q}) - (x_q - \hat{x}_q)] \}  \\
 &= \cov(x_{1-p}, x_{1-q}) - \cov(x_{1-p}, x_q) + \cov(x_p, x_{1-q}) - \cov(x_p, x_q) \\
& \;\;\;\;\;\;   - 2 \cov(x_{0.5},x_{1-q}) + 2\cov(x_{0.5},x_q) 
\end{align*}

%---------------------------------------------------------------------%
\subsection{$\cov(R_{1,p},S_q)$} \label{sec:Cov_rpsq}
%---------------------------------------------------------------------%
\begin{align*}
&\cov(r_{1p},s_q) \\
&= \cov(x_{1-p} - x_p, x_{1-q} + x_q -2x_{0.5}) \\ 
&= E\{[(x_{1-p}- \hat{x}_{1-p}) - (x_p - \hat{x}_p)]  [(x_{1-q}- \hat{x}_{1-q}) + (x_q - \hat{x}_q)- 2 (x_{0.5} - \hat{x}_{0.5})] \}  \\
 &= \cov(x_{1-p}, x_{1-q}) + \cov(x_{1-p}, x_q) -2\cov(x_{1-p}, x_{0.5}) \\
& \;\;\;\;\;\; - \cov(x_p, x_{1-q}) - \cov(x_p, x_q)  +  2\cov(x_p, x_{0.5}) 
\end{align*}
%---------------------------------------------------------------------%
\subsection{$\cov(R_{1,p},R_{1,q})$} \label{sec:Cov_rprq}
%---------------------------------------------------------------------%
\begin{align*}
&\cov(r_{1p},r_{1q})\\
&= \cov(x_{1-p} - x_p, x_{1-q} - x_q) \\
&= E\{[(x_{1-p}- \hat{x}_{1-p}) - (x_p - \hat{x}_p)]  [(x_{1-q}- \hat{x}_{1-q}) - (x_q - \hat{x}_q)] \}\\
&= \cov(x_{1-p},x_{1-q}) - Cov(x_{1-p},x_q) - Cov(x_p, x_{1-q}) + Cov(x_p, x_q)
\end{align*}
To evaluate the variances and covariances of sample quantiles appearing above, we use the first order asymptotic covariance expressions, see \cite[Ch.2]{david-1981},\cite[Ch.7]{Das-2008} and  \citep{prendergast2017large} as described in the beginning of section \ref{sec:ASV}.
